# Supplementary material for: IceDiff: High Resolution and High-Quality Sea Ice Forecasting with Generative Diffusion Prior
Source: arXiv:2410.09111 source file (2024-10-10)
Supplement: Supplementary file 1 [file Compare.tex]

\section{Comparison with Original Scale SIC Map}
To further verify the superiority of our method, we attempt to down-scale the original SIC map and compare IceDiff-GDM with interpolation-based methods and GDP.
FID and Consistency metrics are adopted to measure the faithfulness between the down-scaled model output and the original SIC map.

As shown in \Cref{fig:appn-highres1}, IceDiff successfully captures small-scale structures from the original map.
The generated map not only achieve a better quality but also down-scale with more clear details.
By contrast, both interpolation-based methods and GDP fail to generate rich details and lack fidelity with the original SIC map on the land margin. 

As demonstrated in \Cref{App_metrics1}, IceDiff-GDM outperforms interpolation-based methods and GDP in terms of both FID and Consistency metrics. 
A lower FID and Consistency metrics reflect a more reasonable down-scaling capability, which validates IceDiff-GDM as a promising method for generating down-scaled, detailed, and faithful SIC maps.

\begin{table}[t]\small
\centering
\caption{\textbf{Quantitative comparison between GDM for SIC down-scaling and other methods.}}
% \vspace{-0.3cm}
\resizebox{\textwidth}{!}{
\begin{tabular}{c|c c c| c c}
    \toprule[1pt]
     \multirow{2}{*}{\textbf{Metrics}} &\multicolumn{3}{c|}{Interpolation-based} & \multicolumn{2}{c}{Diffusion-based}\\
     \cmidrule(lr){2-6}

    &Nearest&Bilinear
    &Bicubic&GDP
    &IceDiff-GDM\\
    \midrule
    Fid$\downarrow$&82.07&78.52&56.70&41.39&\textbf{34.77}\\
    Const.$\downarrow$&21.73&19.02&14.17&8.75&\textbf{7.42}\\
    \bottomrule[1pt]

  \end{tabular}
  }
 \label{App_metrics1}
\vspace{-0.3cm}
\end{table}
