# Supplementary material for: IceDiff: High Resolution and High-Quality Sea Ice Forecasting with Generative Diffusion Prior
Source: arXiv:2410.09111 source file (2024-10-10)
Supplement: Supplementary file 2 [file Conditional_Reverse_Process.tex]

\section{Conditional Reverse Process}
\label{Conditional_Reverse_Process}

\begin{figure}[t]
    \centering
    \includegraphics[width=\linewidth]{AnonymousSubmission/LaTeX/Appendix/Figs/grid_illu.pdf}
   % \vspace{-1.3cm}
    \caption{\textbf{Illustration of down-scaling grid.} (a) Visualization of the original and down-scaled grid on 250km x 250km scale. (b) Comparison between the original 25km x 25km grid and down-scaled 6.25km x 6.25km grid. Down-scaling by our IceDiff-GDM could generate fine-grained SIC maps that are consistent with their coarse counterparts.}
    \label{fig:appn-highres1}
\end{figure}

This section aims to provide a detailed derivation of the conditional reverse process formula and prove that the term of $N_2$ in \textbf{Equation (3) in the main text} is a constant.

Previous work \cite{dhariwal2021diffusion} has derived the conditional transformation formula in the reverse process:
\begin{align}
\label{con1} \log_{}{p_\theta(x_{t}|x_{t+1},y)}=\log_{}{(p_\theta(x_{t}|x_{t+1})p(y|x_{t})) }+N_1,
\end{align}
where $N_1$ refers to the conditional distribution $p_\theta(y|x_{t+1})$. Since it isn't dependent on $x_t$, it can be seen as a normalizing constant. 

As to the reverse process of the diffusion model, the posterior $q(x_t|x_{t+1})$ used for sampling is hard to compute. Therefore, we utilize the model with parameter $\theta$ to approximate the conditional probabilities.

\begin{align}
\label{equ1} p_\theta(x_t|x_{t+1})&=\mathcal{N}(\mu_\theta,\Sigma_\theta)\\
\label{equ2} \log_{}{p_\theta(x_t|x_{t+1})}&=-\frac{1}{2}(x_t-\mu_\theta)^T\Sigma_\theta^{-1}(x_t-\mu_\theta)+C_1.
\end{align}
\Cref{equ2} is a direct logarithmic expansion of \Cref{equ1}, where 
\begin{align}
C_1=-\log_{}{(2\pi)^{\frac{n}{2}}(\left | \Sigma_\theta \right |^{\frac{1}{2}} )}=-\frac{n}{2}\log_{}{2\pi}-\frac{1}{2}\log_{}{\left | \Sigma_\theta \right |}
\end{align}

Regarding the another term on the right-hand side of \Cref{con1} $p_\theta(y|x_t)$, it is difficult to calculate directly. 
Hence, Taylor expansion around $x_t=\mu_\theta$ can be used to estimate its value.
By taking the first two terms of its Taylor expansion, we can obtain:
\begin{align}
\log_{}{p_\theta(y|x_t)}&\approx\log_{}{p_\theta(y|x_t)}|_{x_t=\mu_\theta}+ \nonumber\\
&(x_t-\mu_\theta)^T\nabla_{x_t}\log_{}{p_\theta(y|x_t)}|_{x_t=\mu_\theta}\\
\label{con2} &=C_2+(x_t-\mu_\theta)^Tg
\end{align}

Considering integrating \Cref{equ2} and \Cref{con2}, We can obtain:

\begin{align}
&\log_{}{p_\theta(x_t|x_{t+1})p_\theta(y|x_{t})}=\log_{}{p_\theta(x_t|x_{t+1})}+\log_{}{p_\theta(y|x_{t})}\\
&\approx -\frac{1}{2}(x_t-\mu_\theta)^T\Sigma_\theta^{-1}(x_t-\mu_\theta)+(x_t-\mu_\theta)^T+C_1+C_2\\
&=-\frac{1}{2}(x_t-\mu_\theta-\Sigma_\theta g)^T\Sigma_\theta^{-1}(x_t-\mu_\theta-\Sigma_\theta g)+ \nonumber\\
&\frac{1}{2}g^T\Sigma_\theta g+C_1+C_2\\
&=\log_{}{p(z)}+N_2,\quad z\sim \mathcal{N}(\mu_\theta+\Sigma_\theta g,\Sigma_\theta),
\end{align}
where $N_2=\frac{1}{2}g^T\Sigma_\theta g+C_2$ is a constant related to $g$.
