# Supplementary material for: IceDiff: High Resolution and High-Quality Sea Ice Forecasting with Generative Diffusion Prior
Source: arXiv:2410.09111 source file (2024-10-10)
Supplement: Supplementary file 3 [file ablat_model_size.tex]

\section{Ablation Study on FM variants}

We also construct two variants of FM, the number of blocks and multi-heads in each layer is configured as follows:
\begin{align}
    FM_{Small} :& Blocks [2,2,6,2] \nonumber, Heads [2,4,4,8] \nonumber\\
    FM_{Base}  :& Blocks [2,2,18,2], Heads [4,8,16,32], \nonumber
\end{align}
where the last number is the setup in the bottleneck. The performance improves when more blocks and heads are added to FM (as in Table~\ref{tab:abla.hperparam}). Hence we choose to use $FM_{Base}$ model throughout this work to forecast SIC for GDM to perform down-scaling.

%numbers of Swin Transformer Blocks within each layer.
% Ablation : Hyperparameter Variant
\begin{table}[t]\small
  \centering
  \caption{\textbf{Ablation study on the variants of FM in IceDiff}. We compare 2 variants of FM, i.e. Base and Small, to evaluate the impact of different configurations}
  \label{tab:abla.hperparam}
  % \vspace{-0.2cm}
  \resizebox{\textwidth}{!}{
  \begin{tabular}{c|c| c c c c c c}
    \toprule[1pt]
{L.T.} & {Variant}
&RMSE$\downarrow$&MAE$\downarrow$&$R^{2}$$\uparrow$&NSE$\uparrow$&IIEE$\downarrow$&SIE$_{dif}$$\downarrow$\\ 
    \hline
  \multirow{2}{*}{7.D.} &Small&0.0403&0.0083&0.988&0.986&867&0.0538\\
  &Base&\textbf{0.0396}&\textbf{0.0080}&\textbf{0.989}&\textbf{0.987}&\textbf{835}&\textbf{0.0315}\\ 
    \hline

  \multirow{2}{*}{8.W.A.}
  &Small&0.0579&0.0116&0.971&0.966&1383&0.1239\\
  &Base&\textbf{0.0553}&\textbf{0.0112}&\textbf{0.973}&\textbf{0.969}&\textbf{1353}&\textbf{0.0871}\\
    \hline

  \multirow{2}{*}{6.M.A.}
  &Small&0.0696&0.0195&0.901&0.902&2607&0.4744\\
  &Base&\textbf{0.0648}&\textbf{0.0168}&\textbf{0.919}&\textbf{0.913}&\textbf{2016}&\textbf{0.2657}\\
    \bottomrule[1pt]
  \end{tabular}
}
% \vspace{-0.3cm}
\end{table}
