# Supplementary material for: IceDiff: High Resolution and High-Quality Sea Ice Forecasting with Generative Diffusion Prior
Source: arXiv:2410.09111 source file (2024-10-10)
Supplement: Supplementary file 4 [file preliminary.tex]

\subsection{Preliminary}
\label{Preliminary}
Diffusion model is a class of generation model which consists of forward and reverse processes. The forward process is a Markov chain defined as follows:
\begin{align}
q(x_1,\cdots ,x_T|x_0)=\prod_{t=1}^{T} {q(x_t|x_{t-1})}.
\end{align}

The forward process gradually adds Gaussian noise to the training data $x_0$. 
When the noise added at each step is small enough and the diffusion step t is large enough, pure Gaussian noise $x_t\sim \mathcal{N}(0,I)$ can be obtained after $T$ diffusion steps. 
Each diffusion step is defined as follows, where $\beta_t $refers to the variance of the forward process, which can be set as a constant or as a parameter that can be learned by reparameterization. 

\begin{align}
q (x_t|x_{t-1})=\mathcal{N}(x_t;\sqrt{1-\beta_t}x_{t-1},\beta_tI).
\end{align}

The reverse process is the inversion of the forward process, aiming to simulate random noise from the noise distribution of each reverse step and restore data from it.

However, it is difficult to directly obtain the mean and variance of the conditional distribution $p_\theta(x_{t-1}|x_t)=\mathcal{N}(x_{t-1};\mu_\theta(x_t,t),\Sigma_\theta I)$ of the reverse process. 
According to the Bayesian formula, the conditional distribution of the reverse process can be transformed as follows:
\begin{align}
q(x_{t-1}|x_t,x_0)=q(x_t|x_{t-1},x_0)\frac{q({x_{t-1}|x_0})}{q(x_t|x_0)}.\label{diffusion_1}
\end{align}

By directly expanding the three terms at the right end of \Cref{diffusion_1}, the mean $\mu_\theta$ of the reverse process can be represented by the following equation:

\begin{align}
\mu_\theta(x_t,t)=\frac{1}{\sqrt{\alpha_t}}(x_t-\frac{\beta_t}{\sqrt{1-\bar{\alpha}_t}}\epsilon_\theta(x_t,t)).
\end{align}

Among them, $\epsilon_\theta(x_t,t)$ is the noise simulation function obtained from training, which enables the model to simulate and eliminate noise in the data sampled from the reverse process.

Diffusion model uses maximum likelihood estimation to obtain the probability distribution of Markov transition in the reverse process. 
Specifically, the noise prediction function $\epsilon_\theta(x_t,t)$ is trained by optimizing the following denoising objectives.

\begin{align}
E_{\epsilon \sim \mathcal{N(0,I)},t\sim [0,T]}[\left \|\epsilon - \epsilon_\theta(x_t,t) \right \|^2 ].
\end{align}
