# Supplementary material for: IceDiff: High Resolution and High-Quality Sea Ice Forecasting with Generative Diffusion Prior
Source: arXiv:2410.09111 source file (2024-10-10)
Supplement: Supplementary file 5 [file sr_quality.tex]

\section{Additional Visualization Results}
Figure~\ref{fig:appn-highres1} presents the difference between original SIC map and the output of IceDiff-GDM. The downscaled SIC map has a minimum of 6.25km grid length, which is a quarter of the original 25km, and provides more detail at finer-scales.

Figure~\ref{fig:appn-highres2} demonstrates that our IceDiff-GDM is more consistent of the original SIC map than the other two baselines.

Figure~\ref{fig:appn-highres3} provides additional visualization results of three different down-scaling methods. Note that both IceDiff-GDM and GDP are based on diffusion models, a few dark pixels (SIC value close to zero) in the open water area are generated during the denoising process.

\begin{figure*}[t]
    \centering
    \includegraphics[width=\linewidth]{AnonymousSubmission/LaTeX/Appendix/Figs/appn_high_res_1.pdf}
   % \vspace{-1.3cm}
    \caption{\textbf{Down-scaling Quality.} Comparison of SIC map at original scale and down-scaled by three different methods (March 27$^{th}$, 2016).}
    \label{fig:appn-highres2}
\end{figure*}

\begin{figure*}[t]
    \centering
    \includegraphics[width=\linewidth]{AnonymousSubmission/LaTeX/Appendix/Figs/appn_high_res_2.pdf}
   % \vspace{-1.3cm}
    \caption{\textbf{Down-scaling Quality.} Comparison of SIC map at original scale and down-scaled by three different methods.}
    \label{fig:appn-highres3}
\end{figure*}
