# Supplementary material for: IceDiff: High Resolution and High-Quality Sea Ice Forecasting with Generative Diffusion Prior
Source: arXiv:2410.09111 source file (2024-10-10)
Supplement: Supplementary file 6 [file Evaluation_Metrics.tex]

\section{Evaluation Metrics}
\label{Evaluation_Metrics}

FID and Consistency are utilized to evaluate the performance of IceDiff-GDM.

\begin{enumerate}
\item \textbf{FID} \cite{NIPS2017_8a1d6947} is an objective indicator used to evaluate the quality of synthesized images. 
The definition of FID is as follows:
\begin{align}
    FID &= \parallel \mu - \mu_w \parallel^2 + tr(\Sigma + \Sigma_w - 2(\Sigma \Sigma_w)^{\frac{1}{2}}),
\end{align}
where $\mathcal{N}(\mu, \Sigma)$ is the multivariate normal distribution estimated from Inception v3 \cite{szegedy2016rethinking} features calculated from original SIC map and the $\mathcal{N}(\mu_w, \Sigma_w)$ is estimated based on the generated down-scaled SIC map.

\item \textbf{Consistency} is adopted to measure faithfulness to the low-resolution SIC map, which refers to mean squared error (MSE) between the low-resolution SIC map and the down-scaled SIC map undergoing the convolution function. 
\end{enumerate}
